# Supplementary material for: Anomalous metallic phase and reduced critical current in superconducting nanowires due to inverse proximity effect
Source: arXiv:2512.02828 ancillary file (2025-12-02)
Supplement: Supplementary file 1 [file Supplemental_Material.pdf]

# Supplemental Material

# Anomalous metallic phase and suppressed critical current due to inverse proximity effect in superconducting nanowires

G. M. Oliveira,[1,3,*] G. O. Steffensen,[2,3,4,*] I. Casal Iglesias,[1,3] M. Gómez,[1,3] A. Ibabe,[1,3] T.Kanne,[7] J. Nygård,[7] R. Aguado,[4,6] A. Levy Yeyati,[2,3,6] and E. J. H. Lee[1,3,6,†]

[1]*Departamento de Física de la Materia Condensada, Universidad Autónoma de Madrid, Madrid, Spain*

[2]*Departamento de Física Teórica de la Materia Condensada, Universidad Autónoma de Madrid, Madrid, Spain*

[3]*Condensed Matter Physics Center (IFIMAC), Universidad Autónoma de Madrid, Madrid, Spain*

[4]*Instituto de Ciencia de Materiales de Madrid (ICMM), Consejo Superior de Investigaciones Cientificas (CSIC), Sor Juana Ines de la Cruz 3, 28049 Madrid, Spain*

[5]*Center for Quantum Devices, Niels Bohr Institute, University of Copenhagen, Madrid, Spain*

[6]*Laboratorio de Transporte Cuántico, Unidad Asociada UAM/ICMM-CSIC, Madrid, Spain*

[7]*Center for Quantum Devices, Niels Bohr Institute, University of Copenhagen, Copenhagen, Denmark.*

## CONTENTS

S1. Device parameters S3

S2. Additional data S4

A. Power law fitting of the switching current S4

B. Device B S6

C. Device C S7

S3. Usadel Simulations S8

References S11

* These authors have contributed equally to this work.

† eduardo.lee@uam.es

## S1. DEVICE PARAMETERS

| Device | $d_f[nm]$ | $d_c[nm]$ | $t_s[nm]$ | $L[nm]$ | $L_{full}[\mu m]$ | $w[nm]$ | $I_s[\mu A]$ | $I_C^{bulk}[\mu A]$ | $T_C[K]$ | $\xi_0[nm]$ | $R_N[\Omega]$ |
|---|---|---|---|---|---|---|---|---|---|---|---|
| A | 122 | 106 | 8 | 650 | 2.1 | 300 | 27.2 | 151 | 1.25 | 100 | 6.3 |
| B | 122 | 106 | 8 | 690 | 2.3 | 300 | 148 | 154 | 1.17 | 115 | 5.7 |
| C | 143 | 127 | 8 | 500 | 2.1 | 300 | 18.8 | 151 | 1.06 | 110 | 4.4 |

TABLE S1. Summary of device parameters discussed in the main text. The nanowire dimensions, i.e., the full wire diameter, $d_f$, the diameter of the InAs core, $d_c$, and the thickness of the Al shell, $t_s$, were obtained by fits of experimental Little-Parks oscillations to equations (2) and (3) of the main text, using Abrikosov-Gorkov theory. From the same fits, we also extract the superconducting critical temperature, $T_C$, and the superconducting coherence length, $\xi_0$. The distances between inner, $L$, and outer, $L_{full}$, electrical leads and the contact width, $w$, refer to the nominal values employed for the e-beam lithography. The switching current, $I_s$, corresponds to the current at which the resistance of the device becomes finite. It was measured at $T = 30$ mK for devices A and B, and at $T = 255$ mK for device C. The pair-breaking critical current, $I_C^{bulk}$, was estimated using Eq. (1) of the main text. Finally, the normal resistance, $R_N$, was obtained from transport measurements for $I >> I_s$.

## S2. ADDITIONAL DATA

### A. Power law fitting of the switching current

In the main text, fits to $I_s(B)$ and $I_r(B)$ were carried out by employing the power laws in equations (2) and (3). As discussed, a good agreement with the experimental data was achieved by using $\gamma_C = 5/2$ and $\gamma_T = 1$. In Fig. S1, we compare fits to $I_s(B_\perp)$ of device A with $\gamma_C = 5/2$ and $\gamma_C = 3/2$. Clearly, the latter, which is the expected exponent for superconducting wires without the inverse proximity effect, fails to capture the dependence of the switching current for higher applied fields. The exponent $\gamma_C = 5/2$ is corroborated by Usadel calculations of inversely proximitized wires.

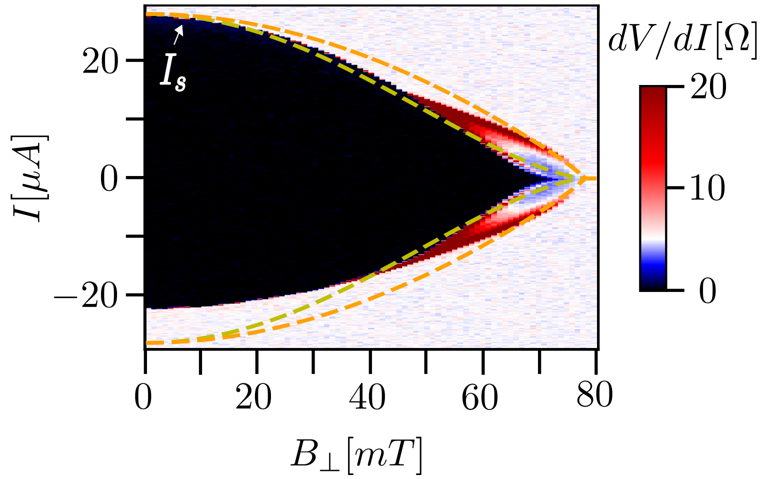


FIG. S1. **Comparison of $\gamma_C = 3/2$ or $5/2$ for fitting the switching current**. Fits to $dV/dI(I, B_\perp)$ of device A (same data as Fig. 2(a) in the main text) using $\gamma_C = 3/2$ (orange dashed line) and $\gamma_C = 5/2$ (yellow dashed line).

In Fig. S2, we plot as yellow dashed lines the $I_s(B_\parallel)$ curves calculated using Abrikosov-Gorkov theory, $\gamma_C = 3/2$, and the parameters extracted by fitting the data in Fig. S1, for $B_\perp = 0, 46$, and 60 mT. While a good agreement is obtained for $B_\perp = 0$, substantial discrepancies appear with increasing $B_\perp$.

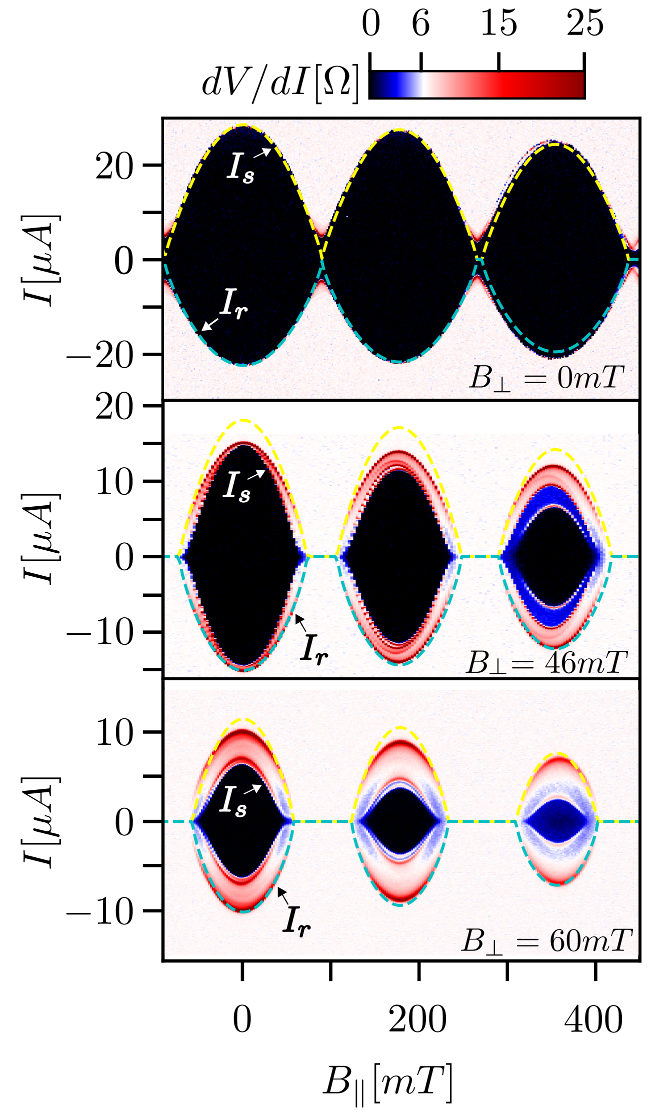


FIG. S2. **Fits to Little-Parks oscillations using** $\gamma_C = 3/2$. Fits to $I_s(B_\parallel)$ (yellow dashed lines) and $I_r(B_\parallel)$ (blue dashed lines) of device A taken at $B_\perp = 0, 46$, and 60 mT (same data as Fig. 4(a) in the main text) using $\gamma_C = 3/2$ and $\gamma_T = 1$.

## B. Device B

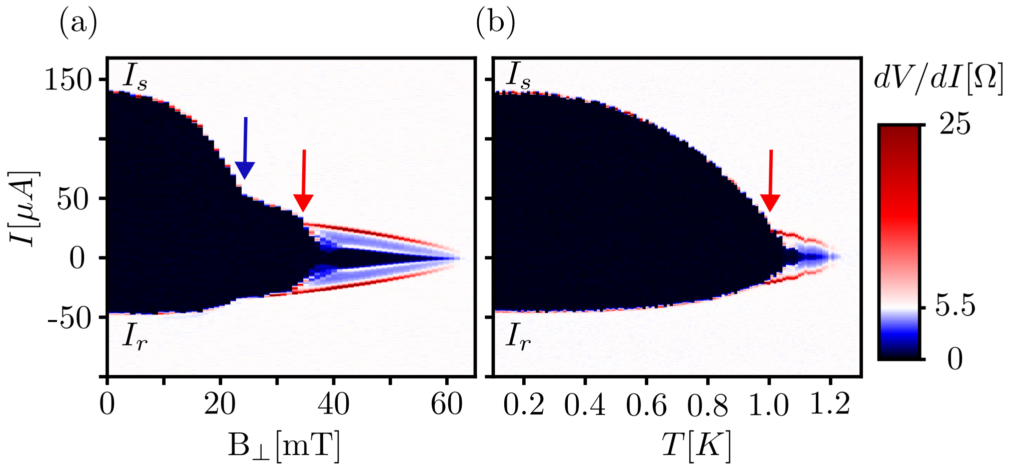


FIG. S3. **Supplementary measurements for device B.** $dV/dI(I)$ measurements as a function of **(a)** magnetic field applied perpendicular to the nanowire axis, and **(b)** bath temperature. Here, the $B_\perp$- and $T$-dependencies are more intricate as the fabricated superconducting leads transition to the normal state in the range of the measurements. Indeed, in panel (a), we observe such a transition at $B_\perp \approx 25$ mT (blue arrow). For higher fields, the behavior is similar to that observed in device A with a transition from the weak to the strong IPE regimes at $B_\perp \approx 35$ mT (red arrow). In panel(b), we also observe the transition from weak to strong IPE at $T \approx 1.1$ K (red arrow), approximately coinciding with the superconducting transition temperature of the fabricated Ti/Al leads.

### C. Device C

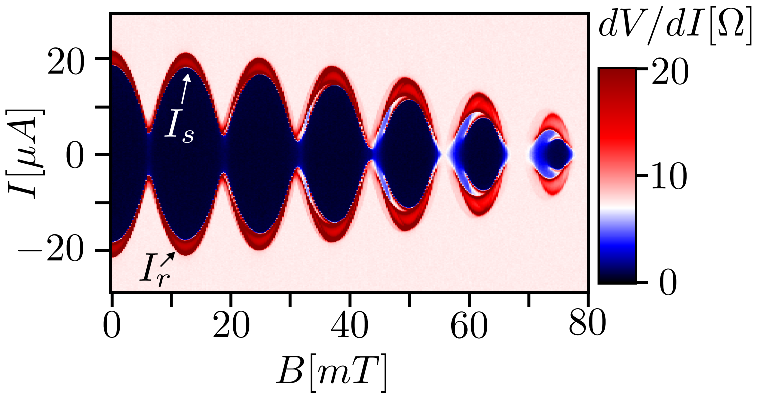


FIG. S4. **Supplementary measurement for device C.** $dV/dI(I, B)$ measurement displaying Little-Parks oscillations of $I_s$ and $I_r$. Here, the device was measured in a system with a single-axis coil. As a result, the applied magnetic field has a small angle with respect to the nanowire axis. Note the absence of a weak IPE regime throughout the measurement, indicating that, owing to a stronger inverse proximity effect, this device is able to stabilize the $\mathcal{N}_\mathcal{S}$ phase even at zero magnetic field.

## S3. USADEL SIMULATIONS

In this section, we describe the Usadel theory [1, 2] used to solve 1D models of the superconducting wire, including effects of inverse proximity from coupling to a metallic lead. This theory describes superconductivity in the diffusive limit, where the mean-free path, $l \ll \xi_{BCS}$, with $\xi_{BCS} = \hbar\nu_F/\pi\Delta_{BCS}$ denoting the BCS coherence length, $\Delta_{BCS}$ the BCS gap, and $\nu_F$ the fermi velocity. In this limit, the difussive dynamics is captured by the coefficient $D = \nu_F l/3$, and the effective coherence length is given by $\xi_0 = \sqrt{\pi\xi_{BCS} l/3}$. The principal Usadel diffusion equation is,

$$\frac{\hbar D}{2}\nabla \cdot \nabla\theta + \left[\omega_n + \frac{D}{2\hbar}\mathbf{q}^2\cos\theta\right]\sin\theta + \Delta\cos\theta, \tag{1}$$

where $\mathbf{q} = \nabla\phi + 2\pi\mathbf{A}/\Phi_0$ denotes the momentum of the condensate, composed of a phase gradient, $\nabla\phi$, and the vector gauge field, $\mathbf{A}$, in units of flux quantum $\Phi_0$. We use Matsubara frequencies $\omega_n = (1 + 2n)\pi k_B T$, and denote the local pairing parameter by $\Delta$, which is typically reduced by IPE and finite $\mathbf{q}$ such that $\Delta \leq \Delta_{BCS}$. Lastly, $\theta$ denotes the pairing angle, such that the normalized Usadel Greens function is given by,

$$G = \begin{pmatrix} \cos\theta & i\sin\theta \\ -i\sin\theta & -\cos\theta \end{pmatrix}, \quad G^2 = 1. \tag{2}$$

One can verify that for a homogeneous, $\nabla \cdot \nabla\theta = 0$, superconductor at rest, $\mathbf{q}^2 = 0$, this yields the usual BCS Greens function. To reduce Eq. (1) to a 1D equation, we recast $D = \frac{\xi_0^2\Delta_{BCS}}{\hbar}$ and note that $\xi_0$ is the length scale of $\theta$ variations. Assuming that the nanowire is approximately cylindrical and Al thickness $t_S \ll \xi_0$, the pairing angle $\theta$ will be constant as a function of wire radius. Further assuming that the Al shell is symmetric around the nanowire, and the metallic leads are equally connected to all shell facets, $\theta$ will also be constant around the wire. Thus, $\theta(x)$ only depends on the coordinate along the wire, $x$, corresponding to a 1D system. Next, we assume the momentum term can be separated into three pair-breaking components,

$$\frac{D}{2\hbar}\mathbf{q}^2 = \alpha = \alpha_\phi + \alpha_\parallel + \alpha_\perp, \tag{3}$$

with $\alpha_\phi = \frac{D}{2\hbar}\left(\frac{\partial\phi}{\partial x}\right)^2$ capturing the supercurrent running along the wire, $\alpha_\parallel$ the supercurrent running around the wire from the little-park effect, and $\alpha_\perp$ the pair-breaking from field perpendicular to the wire, given by Eq. (5) and Eq. (6) in the main text respectively. Note,

that for simplicity we have neglected cross terms of $\alpha_\phi$ and $\alpha_\perp$ of the form $\frac{\partial\phi}{\partial x}\mathbf{x}\cdot A_x\mathbf{x}$. Including these terms would require solving a 2D problem with angular dependence of $\alpha$ and $\theta$, going beyond our current scope. Lastly, to include the inverse proximity effect, we assume that the thin shell is coupled to a much larger metallic lead, such that superconducting proximity onto the metal is negligible, so its pairing angle is $\theta_N = 0$. Using typical Kupriyanov-Lukichev boundary conditions [3, 4] and this assumption, we find,

$$\sigma_S \nabla_n \theta = \frac{\sin\theta}{R_I A_I}, \tag{4}$$

with $\sigma_S$ denoting the shells conductivity, $\nabla_n$ the gradient normal to the interface, $R_I$ and $A_I$ the resistance and area of the superconductor-to-normal interface. Using this, we integrate Eq. (1) along the interface to obtain our 1D Usadel model,

$$\frac{\hbar D}{2}\frac{\partial^2\theta}{\partial x^2}(x) + [\omega_n + \Pi F(x) + \alpha(x)\cos\theta(x)]\sin\theta(x) + \Delta(x)\cos\theta(x). \tag{5}$$

The boundary condition is now captured by a constant, $\Pi = \Delta_{BCS}\frac{R_N}{R_I}\frac{\xi_0^2}{wL}$, which apart from $R_I$ is fully determined from fitted values presented in table S1. The function $F(x)$ is either 1 or 0, thus defining the range in $x$ that is contacted by a metal. Next, to solve Eq. (5) we need to insure self-consistency in both the local pairing-parameter and the current [5, 6], which is captured by the following equations,

$$0 = \Delta(x)\ln\left(\frac{T}{T_{c0}}\right) + 2\pi k_B T \sum_{n\geq 0}\left(\frac{\Delta(x)}{\omega_n} - \sin\theta(x)\right), \tag{6}$$

$$I(x) = \frac{\sqrt{2}d}{eR_N\xi_0}\sqrt{\frac{\alpha_\phi(x)}{\Delta_{BCS}}}\pi k_B T\sum_{n\geq 0}\sin^2\theta(x), \tag{7}$$

where $k_B T_{c0} = \Delta_{BCS}/1.764$. With these equations we solve Eq. (5) on a 1D discreet grid in $x$, including Matsubara frequencies up to a chosen $n_{max}$ that insures convergence of pairing, $\Delta(x)$. We then enforce constant current, $I(x) = \text{const}$, as a boundary condition and solve for $\theta(x, \omega_n)$, $\Delta(x)$, and $\alpha_\phi(x)$ self-consistently. To provide some intuition, consider that pair-breaking, $\alpha_\phi(x)$, appearing from a finite phase gradient, $\partial_x\phi(x)$, reduces the local pairing $\Delta(x)$, which lowers the current, $I(x)$. One then has to increase $\partial_x\phi$ to insure $I(x) = \text{const}$ which further affects $\Delta$ in a self-consistent manner, which is what we are solving for at each $x$. Note that all dependence of $x$ stems from $F(x)$, and for $F(x) = \text{const}$ the system becomes homegenous with $\partial_x^2\theta = 0$ in Eq. (5).

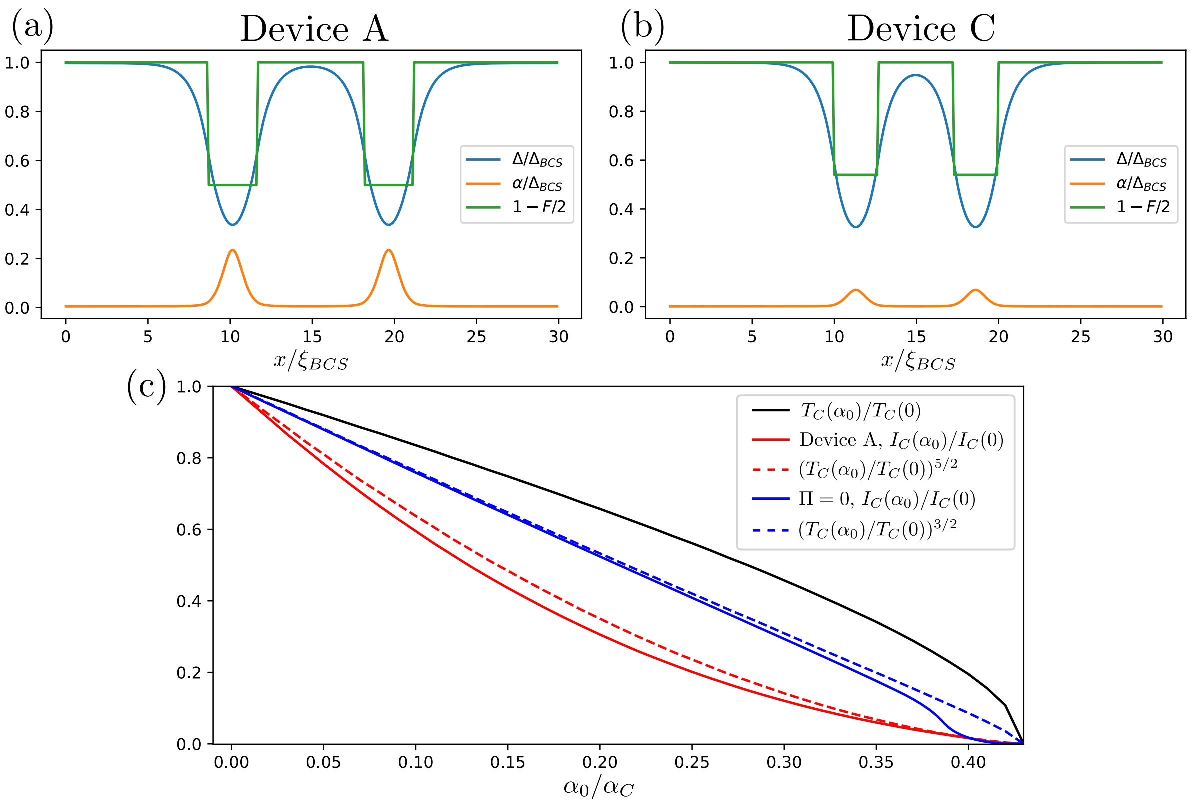


FIG. S5. (a, b) Self-consistent $\Delta(x)$ and $\alpha(x)$ profiles obtained from Eq. (5) using parameters for device A and device B (see table S1) for $T_B = 0.1T_{c0}$ and (a) $I = 0.1I_C^{bulk}$, (b) $I = 0.05I_C^{bulk}$. The green lines highlight the position of the metallic contacts. (c) Scalings of critical current obtained from Eq. (5) with pair-breaking, $\alpha_0 = \alpha_{\|} + \alpha_{\perp}$, from magnetic field fitted to power laws of $T_C(\alpha_0)/T_C(0)$. The critical pair-breaking at which $\Delta = 0$ is denoted by $\alpha_C$.

In Fig S5 (a, b) we show solutions of the Usadel equations for device A and device C, using the fitted values of $R_I^A = 0.25\Omega$ and $R_I^C = 0.22\Omega$. At the edges, $L_{min}$ and $L_{max}$, we assumed bulk boundary conditions corresponding to $\partial_x^2\theta = 0$ in Eq. (5). The values of $L_{min}$ and $L_{max}$ were chosen sufficiently large so as to assure convergence. As can be seen in Fig. S5 (a, b), the system behaves as a Josephson junction with a phase gradient, captured by $\alpha$, peaking at the weakspots formed under the metallic contacts. To find the critical current we increase the current, $I$, until no self-consistent solution exists heralded by a divergence of $\alpha$ around the weakspots. We denote by $I_C(B)$ the value of $I$ at this threshold, and we find $R_I$ by fitting this value to measurements in Fig. 3 (c, d) of the main text. To obtain the critical temperature, we increase $T$ until no self-consistent solution exists, keeping the current fixed at $I = 0.001I_C^{bulk}$ to ensure numerical stability. These simulations demonstrate

that a reduction of $I_C$ from the bulk value of $I_C^{bulk}$ is compatible with realistic values of $R_I$, and consistent with the measured reductions of $T_C$. Another prediction of our Usadel model is a change of the power law scaling with $T_C(B)/T_C(0)$ of the critical current, which is shown in Fig. S5 (c). Here, one can compare the predicted scaling with a 3/2 exponent for homogeneous systems [5], $\Pi = 0.0$, to a scaling with a 5/2 exponent arising from the parameters for Device A.


[1] K. D. Usadel, Generalized diffusion equation for superconducting alloys, Physical Review Letters **25**, 507–509 (1970).

[2] W. Belzig, F. K. Wilhelm, C. Bruder, G. Schön, and A. D. Zaikin, Quasiclassical green's function approach to mesoscopic superconductivity, Superlattices and Microstructures **25**, 1251–1288 (1999).

[3] M. Y. Kupriyanov and V. F. Lukichev, Influence of boundary transparency on the critical current of "dirty" ss's structures, Sov. Phys. JETP **67**, 1163 (1988).

[4] Y. V. Fominov and M. V. Feigel'man, Superconductive properties of thin dirty superconductor–normal-metal bilayers, Phys. Rev. B **63**, 094518 (2001).

[5] J. Romijn, T. M. Klapwijk, M. J. Renne, and J. E. Mooij, Critical pair-breaking current in superconducting aluminum strips far belowtc, Physical review. B, Condensed matter **26**, 3648–3655 (1982).

[6] D. Y. Vodolazov, A. Y. Aladyshkin, E. E. Pestov, S. N. Vdovichev, S. S. Ustavshikov, M. Y. Levichev, A. V. Putilov, P. A. Yunin, A. I. El'kina, N. N. Bukharov, and A. M. Klushin, Peculiar superconducting properties of a thin film superconductor–normal metal bilayer with large ratio of resistivities, Superconductor Science and Technology **31**, 115004 (2018).
